# Supplementary material for: A Regret Minimization Approach to Multi-Agent Control
Source: arXiv:2201.13288 source file (2022-02-25)
Supplement: Supplementary file 1 [file control_sharing.tex]

\section{Shared Controls}\label{sec:shared_controls}
In this section, we provide a brief justification of the multi-agent control information model involving the sharing of controls between agents. While this does not preclude regret guarantees with other restrictions on policy classes, or different information models, we show that the current set of assumptions of Theorem~\ref{thm:ctrl_regret} is incompatible with unobserved controls. The core idea is that to minimize regret, controls need to be disambiguated, but observations and cost alone are not enough to do this.  This construction assumes that the control algorithm is deterministic and proper in the sense that each agent must play via a policy in it's comparator class. The key trick is that because each agent is agnostic of the policy parameterization of other players, the policy class can be designed adversarially.

\begin{figure}[h]
\centering
\vskip5mm
\setlength{\unitlength}{0.13cm}
\begin{center}\begin{picture}(54,29)(0,31)
\thicklines
\put(24,54){\framebox(16,12){$\mathbf S$}}

\put(26,42){\framebox(12,8){$\cC_1 $}}
\put(26,30){\framebox(12,8){$\cC_2 $}}

\put(17,64.5){$w, e$}
\put(16,64){\vector(1,0){8}}

\put(43,64.5){$x$}
\put(40,64){\vector(1,0){7}}

\put(40,47){$y^1$}
\put(44,56){\line(0,-1){10}}
\put(40,56){\line(1,0){4}}
\put(44,46){\vector(-1,0){6}}

\put(40,35){$y^2$}
\put(40,60){\line(1,0){6}}
\put(46,60){\line(0,-1){26}}
\put(46,34){\vector(-1,0){8}}

\put(22,46.5){$u^1$}
\put(26,46){\line(-1,0){7}}
\put(19,56){\vector(1,0){5}}
\put(19,46){\line(0,1){10}}

\put(22,34.5){$u^2$}
\put(26,34){\line(-1,0){9}}
\put(17,34){\line(0,1){26}}
\put(17,60){\vector(1,0){7}}

\end{picture}\end{center}
\caption{Diagram of a $2$ agent System $\mathbf S$ executing dynamics from \eqref{eq:gen_dynamics} with agents $\cC_1, \cC_2$ \bf{without sharing controls}.}
\label{fig:multiagent_system}
\end{figure}

\begin{theorem}\label{thm:control_sharing}
In the modified information model, where controls are not shared between agents, there is a multi-agent control problem where Assumptions~\ref{assumption:bounded_nat_y},~\ref{assumption:cost},~\ref{assumption:dist_policy} hold and Assumptions~\ref{assumption:burn-in}, ~\ref{assumption:convexity} holds with burn-in $1$, horizon $1$ and error $0$, where average regret must be $\regret_T = \Omega(1)$ for deterministic agents that always play a control $u^i_t$ via a policy $\pi^i_t \in \Pi^i$.
\end{theorem}
\begin{proof}
We consider a three agent LDS with scalar states/controls, static quadratic costs, and zero disturbance defined by the following
\begin{align*}
    x_{t+1} = 0 \cdot x_t + 0 u_t + w_t = 0\\
    c_t(x_t, u_t)= (u^{1}_t - u^{2}_t)^2 + (u^{3})^2
\end{align*}

We consider $\Pi^{1}$ to be a class of constant policies defined by a constant action $\pi^1 \in [0,1]$. Both $\Pi^2$ and $\Pi^3$ are defined to be open loop trajectories.   $\Pi^2,\Pi^3$ are defined constructively given the deterministic agent for $1$ in the following way. We construct two possible trajectories:
\begin{enumerate}
    \item $\forall t, u^{2}_t = 0, u^{3}_t = \sqrt{1 - (u^{1}_t - u^{2}_t)^2}, $
    \item $\forall t,  u^{2}_t =1, u^{3}_t = \sqrt{1 - (u^{1}_t - u^{2}_t)^2}$
\end{enumerate}

The cost is always $1$ on both trajectories and state is always $0$ so $u^{1}_t$, produced by a deterministic algorithm must be the same in both of these trajectories.  The average regret of the first trajectory is $\frac{1}{T}\sum_{t=1}^T (u^1_t)^2$ while the average regret of the second trajectory is $\frac{1}{T}\sum_{t=1}^T (u^1_t -1)^2$.  One of these must be $> \frac{1}{4}$ and hence, we can choose the open loop policies for agents $2$ and $3$ to ensure a constant average regret.
\end{proof}
